# Supplementary material for: SmartFL: Semantics Based Probabilistic Fault Localization
Source: arXiv:2503.23224 source file (2025-04-03)
Supplement: Supplementary file 1 [file appendix.tex]

% \newpage
\appendix[Details of Inference Optimization Deduction]
% \section{Details of Inference Optimization Deduction}
\label{appendix}
For simplicity, we use 1 to denote \textit{true} and 0 to denote \textit{false}.

\begin{align*}
    \begin{split}
    \mu_{a \rightarrow v}(1) & = \sum_{X} f(1,X) \prod_{v_i \in V} \mu_{v_i \rightarrow a}(x_i) \\
     & = f(1,1,\dots,1) \prod_{v_i \in V} \mu_{v_i \rightarrow a}(1) + \sum_{\exists x_i \in X: x_i = 0} f(1,X) \prod_{v_i \in V} \mu_{v_i \rightarrow a}(x_i)\\
     & = 1 \cdot \prod_{v_i \in V} \mu_{v_i \rightarrow a}(1) + p_0 \sum_{\exists x_i \in X: x_i = 0} \prod_{v_i \in V} \mu_{v_i \rightarrow a}(x_i)  \\
     & = \prod_{v_i \in V} \mu_{v_i \rightarrow a}(1) + p_0 \sum_{X} \prod_{v_i \in V} \mu_{v_i \rightarrow a}(x_i) - p_0 \prod_{v_i \in V} \mu_{v_i \rightarrow a}(1)\\
     & = \prod_{v_i \in V} \mu_{v_i \rightarrow a}(1) + p_0 \prod_{v_i \in V} (\mu_{v_i \rightarrow a}(0) + \mu_{v_i \rightarrow a}(1)) - p_0 \prod_{v_i \in V} \mu_{v_i \rightarrow a}(1) \\
     & = \prod_{v_i \in V} \mu_{v_i \rightarrow a}(1) + p_0 - p_0 \prod_{v_i \in V} \mu_{v_i \rightarrow a}(1)\\
     & = (1-p_0) \prod_{v_i \in V} \mu_{v_i \rightarrow a}(1) + p_0\\
    \end{split}
\end{align*}
